# Supplementary material for: Mechanism for Strong Chimeras
Source: arXiv:2101.12230 ancillary file (2021-03-08)
Supplement: Supplementary file 1 [file Supplemental_Material.pdf]

# Supplemental Material

*Mechanism for Strong Chimeras*
*Yuanzhao Zhang and Adilson E. Motter*

## CONTENTS

S1. Strong chimeras in coupled logistic maps 1

S2. Strong chimeras in continuous-time dynamical systems 2

S3. Robustness against oscillator heterogeneity 3

S4. Nature of the desynchronization transition 4

S5. Characteristics of the effective input and its impact on stability 5

## S1. STRONG CHIMERAS IN COUPLED LOGISTIC MAPS

Here, we show that the same mechanism described in the main text gives rise to strong chimeras in networks and oscillator models other than the ones investigated in Figs. 2 and 5. In Fig. S1, we consider coupled logistic maps and show their transition from coherence to incoherence through chimera states. The system can be described by the dynamical equation

$$x_i^{t+1} = \left\{ r x_i^t (1 - x_i^t) - K \sum_{j=1}^{N} L_{ij} x_j^t (1 - x_j^t) \right\} \bmod 1, \quad i = 1, \dots, N, \tag{S1}$$

where $\boldsymbol{L} = \{L_{ij}\}$ is the Laplacian matrix representing a two-cluster network with nearest-neighbor intracluster coupling and all-to-all intercluster coupling [Fig. S1(a)].

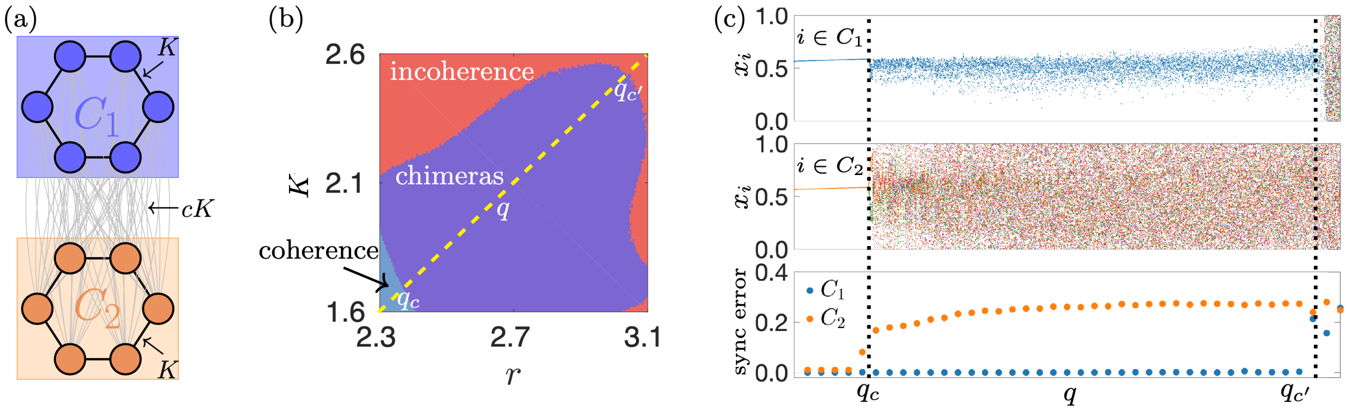


FIG. S1. Analog of Fig. 2 in the main text for a two-cluster network of logistic maps. The value of $c$ is again set to 0.2. The dynamics in the top and middle panels in (c) are obtained by varying $q$ quasi-statically along the dashed line in (b) ($r = 2.3 + 8 \times 10^{-5} t$, $K = 1.6 + 10^{-4} t$ for $10^4$ iterations). The bottom panel in (c) shows the time-averaged synchronization errors in the two clusters for fixed values of $q$. Each data point is averaged over $10^3$ iterations, and the final state from the previous data point is used as the initial condition for the next data point (with increased $q$). The orange points are shifted slightly to avoid complete overlap with the blue points below $q_c$.

## S2. STRONG CHIMERAS IN CONTINUOUS-TIME DYNAMICAL SYSTEMS

We further demonstrate that incoherence-stabilized coherence is not limited to discrete maps and it can also give rise to strong chimeras in continuous-time dynamical systems. For this purpose, we consider the multilayer network depicted in Fig. S2(a), where the intracluster and intercluster coupling are mediated by different types of interactions. Each layer consists of six identical Lorenz oscillators interacting through the coupling function $\boldsymbol{H}_1 = (0,0,z)^\intercal$. In addition, the two layers are all-to-all coupled through the coupling function $\boldsymbol{H}_2 = (0,0,x)^\intercal$. The oscillators in the first layer are thus described by the equations

$$\begin{aligned}
\dot{x}_i^{(1)} &= \alpha(y_i^{(1)} - x_i^{(1)}),\\
\dot{y}_i^{(1)} &= x_i^{(1)}(\rho - z_i^{(1)}) - y_i^{(1)},\\
\dot{z}_i^{(1)} &= x_i^{(1)}y_i^{(1)} - \beta z_i^{(1)} + K(z_{i+1}^{(1)} + z_{i-1}^{(1)} - 2z_i^{(1)}) + cK\sum_{j=1}^{6}(x_j^{(2)} - x_i^{(1)}),
\end{aligned} \tag{S2}$$

where the superscripts identify the layers and we set $\alpha = 10$, $\beta = 2$, and $c = 0.2$, leaving the parameters $\rho$ and $K$ to be varied. The oscillators in the second layer are described by similar equations.

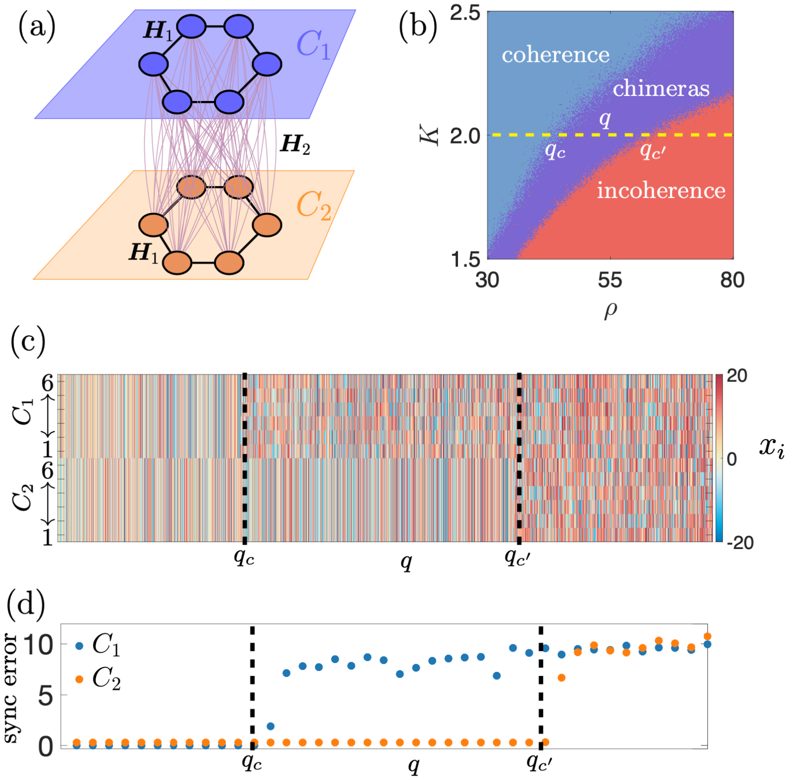


FIG. S2. Chimera states in continuous-time dynamical systems. (a) Multilayer network of Lorenz oscillators with different intralayer and interlayer interactions, given by $\boldsymbol{H}_1$ and $\boldsymbol{H}_2$, respectively. (b) Diagram in the ($\rho$,$K$) plane marking the regions for which the system exhibits coherence (cyan), chimeras (purple), and incoherence (red) according to our linear stability analysis. (c) State transitions as parameter $q$ is varied quasi-statically along the dashed line in (b) ($\rho = 30 + 5\times10^{-3}t$, $K = 2$ for $10^4$ time units). Incoherence-stabilized coherence gives rise to strong chimeras as the system transitions from coherence to incoherence. (d) Time-averaged synchronization errors in the two clusters for fixed values of $q$. Each data point is averaged over $10^3$ time units, and the final state from the previous data point is used as the initial condition for the next data point for increasing $q$. The orange points are shifted slightly to avoid complete overlap with the blue points below $q_c$.

## S3. ROBUSTNESS AGAINST OSCILLATOR HETEROGENEITY

Our results are robust to the presence of oscillator heterogeneity, which we demonstrate in Fig. S3 by introducing random mismatches with a standard deviation of $10^{-3}$ (drawn from a Gaussian distribution) to the parameter $\beta$ for the same transitions studied in Fig. 2.

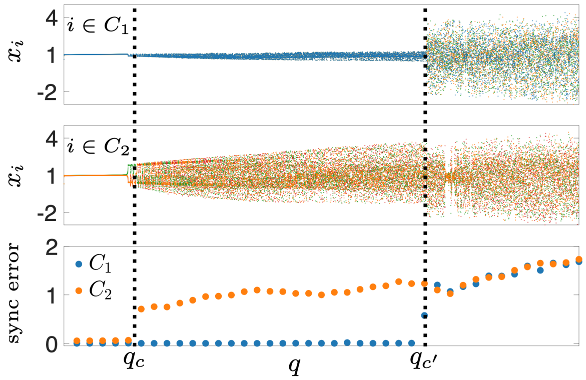


FIG. S3. Analog of Fig. 2(c), with oscillator heterogeneity incorporated into the simulation to mimic a realistic aspect of experimental conditions.

## S4. NATURE OF THE DESYNCHRONIZATION TRANSITION

Consider the two-cluster networks analyzed in the main text, where the clusters are identical and connected to each other through all-to-all coupling of strength $cK$. The clusters, $C_1$ and $C_2$, can be allowed to have arbitrary size and network structure. In such systems, as a bifurcation parameter is varied, global synchronization can lose stability through either intercluster desynchronization ($C_1$ and $C_2$ go to different states) or intracluster desynchronization ($C_1$ and/or $C_2$ desynchronize within themselves). In both cases, stability is determined by the master stability function $\widetilde{\Lambda}(\alpha, \beta)$.

For diffusively coupled oscillators, $\widehat{\lambda}_1 = -cn$ for the intercluster case and $\widehat{\lambda}_i = -\lambda_i - cn$ for the intracluster case, where we used that $\mu = -cn$ and that $\lambda_i$ are the eigenvalues of the Laplacian matrix of the cluster for $i = 2, ..., n$. In this analysis, $K\mu h(s^t) + I(t) = 0$ and thus $\Gamma_s = \Gamma_0$, where $\Gamma_0$ is the Lyapunov exponent of an isolated oscillator defined by $f$. Thus, the stability of the global synchronization state requires $\alpha_1 = Kcn$ (intercluster) and $\alpha_i = Kcn + K\lambda_i$ for $i = 2, \ldots, n$ (intracluster) all to be in the negative region of $\widetilde{\Lambda}(\alpha_i, \beta)$.

The stability conditions then take the form

$$(-\beta + Kcn)^2 < e^{-2\Gamma_0} \quad \text{for intercluster,} \tag{S3}$$

$$(-\beta + Kcn + K\,\mathrm{Re}\lambda_i)^2 + (K\,\mathrm{Im}\lambda_i)^2 < e^{-2\Gamma_0} \quad \text{for intracluster,} \tag{S4}$$

where $\mathrm{Re}\,\lambda_i$ and $\mathrm{Im}\,\lambda_i$ are the real and imaginary parts of the eigenvalue, respectively. Equation (S4) represents the condition in Eq. (6), whereas Eq. (S3) corresponds to the perturbation mode parallel to the cluster synchronization manifold omitted in Eq. (6). Since $c$ and $\mathrm{Re}\,\lambda_i$ are nonnegative for the systems we consider, it follows that the condition in Eq. (S4) is the first to be violated as $K$ is increased beyond the stability region, and thus the stability of global synchronization is first lost through intracluster desynchronization. Analogous description applies to the bifurcation parameter $q$ in Fig. 2(b).

The condition in Eq. (S3) is violated first when the stability boundary is reached by decreasing $K$, meaning that for small $K$ stability can be lost through intercluster desynchronization if $\beta^2 > e^{-2\Gamma_0}$. Here, we focus on intracluster desynchronization transitions as induced by any bifurcation parameter, given our focus on chimeras, but our results also apply to transitions involving intercluster desynchronization as well as intercluster desynchronization followed by intracluster desynchronization.

The only difference in the latter case is that, if intercluster desynchronization happens first and is followed by intracluster desynchronization (e.g., small $K$ for chaotic oscillators) giving rise to a chimera, then the stability analysis has to be repeated twice since now $s^t$ changes due to nonvanishing $K\mu h(s^t) + I(t)$ between the two desynchronizations. The analysis of the transition to the chimera is then to be performed in two steps by updating $s^t$ and thus $\Gamma_s$.

## S5. CHARACTERISTICS OF THE EFFECTIVE INPUT AND ITS IMPACT ON STABILITY

For a more systematic understanding of the interaction between the two clusters, we vary the intercluster coupling strength by varying $c$ while the other parameters are kept fixed. We first calculate the mean $\nu$ and standard deviation $\sigma$ of the effective input [Fig. S4(a)]. As $c$ is increased from zero, $\nu$ steadily decreases while $\sigma$ increases. Figure S4(b) shows the resulting LTLE for synchronization in the coherent cluster when this cluster is subject to Gaussian white noise input or effective input from the incoherent cluster. For each value of $c$, the mean and standard deviation of the noise input are set respectively to the values of $\nu = \nu(c)$ and $\sigma = \sigma(c)$ from Fig. S4(a). Both forms of input lead to the stabilization of synchronization for intermediate intercluster coupling strength, which is to be contrasted with the unstable state obtained if the other cluster is set to the same coherent state [shown in Fig. S4(b) as a reference]. This suggests that the stabilization effect of a common driving signal is relatively insensitive to the details of the signal, as long as the mean and standard deviation of the signal are suitable.

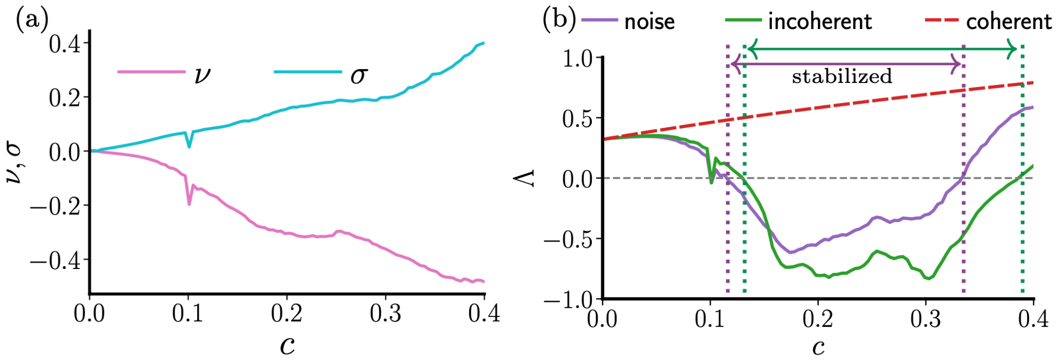


FIG. S4. Dependence of effective input and synchronization stability on intercluster coupling strength. (a) Mean $\nu$ and standard deviation $\sigma$ of the effective input from the incoherent cluster as the coupling parameter $c$ is varied. (b) LTLE of the coherent cluster as a function of $c$ for noise input (purple), effective input based on direct simulation of the incoherent cluster (green), and no input (red). The system is the same as in Figs. 2–4 for $\beta = 1.2$ and $K = 1.2$.
